# Supplementary material for: Temporal Graph Convolutional Networks for Automatic Seizure Detection
Source: arXiv:1905.01375 source file (2019-05-03)
Supplement: Supplementary file 1 [file appendix.tex]

\appendix
\section*{Appendix}

\begin{table}[htbp]
\centering 
  \caption{Set of EEG leads analyzed, and how they were arranged for several models.}
\begin{tabular}{|l|l|l|l|}
\hline
\multicolumn{1}{|c|}{Leads analyzed}                                                                                                                & \multicolumn{1}{c|}{\begin{tabular}[c]{@{}c@{}}Inputs for TCNN\\ with montage\end{tabular}}                                                                                                                                                                         & \multicolumn{1}{c|}{\begin{tabular}[c]{@{}c@{}}Input ordering for\\ 2D TCNN\end{tabular}}                                                                                                          & \multicolumn{1}{c|}{\begin{tabular}[c]{@{}c@{}}Input ordering for 2D\\ TCNN with montage\end{tabular}}                                                                                                                                                              \\ \hline
\begin{tabular}[t]{@{}l@{}}C3\\ C4\\ Cz\\ F3\\ F4\\ F7\\ F8\\ Fz\\ FT9\\ FT10\\ Fp1\\ Fp2\\ O1\\ O2\\ P3\\ P4\\ P7\\ P8\\ Pz\\ T7\\ T8\end{tabular} & \begin{tabular}[t]{@{}l@{}}Fp1 - F7\\ F7 - T7\\ T7 - P7\\ P7 - O1\\ \\ Fp1 - F3\\ F3 - C3\\ C3 - P3\\ P3 - O1\\ \\ Fz - Cz\\ Cz - Pz\\ \\ Fp2 - F4\\ F4 - C4\\ C4 - P4\\ P4 - O2\\ \\ Fp2 - F8\\ F8 - T8\\ T8 - P8\\ P8 - O2\\ \\ FT9 - F7\\ FT10 - F8\end{tabular} & \begin{tabular}[t]{@{}l@{}}Fp1\\ F7\\ T7\\ P7\\ O1\\ \\ Fp1\\ F3\\ C3\\ P3\\ O1\\ \\ Fz\\ Cz\\ Pz\\ \\ Fp2\\ F4\\ T4\\ P4\\ O2\\ \\ Fp2\\ F8\\ T8\\ P8\\ O2\\ \\ FT9\\ F7\\ FT10\\ F8\end{tabular} & \begin{tabular}[t]{@{}l@{}}Fp1 - F7\\ F7 - T7\\ T7 - P7\\ P7 - O1\\ \\ Fp1 - F3\\ F3 - C3\\ C3 - P3\\ P3 - O1\\ \\ Fz - Cz\\ Cz - Pz\\ \\ Fp2 - F4\\ F4 - C4\\ C4 - P4\\ P4 - O2\\ \\ Fp2 - F8\\ F8 - T8\\ T8 - P8\\ P8 - O2\\ \\ FT9 - F7\\ FT10 - F8\end{tabular} \\ \hline
\end{tabular}
\end{table}

\begin{table}[htbp]
  \centering 
  \caption{Lead groups for brain regions. These groups were used for generating Figure \ref{fig:dropout}B from the sequence dropout experiment.} 
  \begin{tabular}{|c|c|}\hline
     & Number of seizures\\ \hline
    Left frontal & Fp1, F3, Fz\\ \hline
    Right frontal & Fp2, F4, Fz\\ \hline
    Left temporal & F7, T7, FT9\\ \hline
    Right temporal & F8, T8, FT10\\ \hline
    Left parietal & P7, P3\\ \hline
    Right parietal & P8, P4\\ \hline
    Left occipital & O1, P7\\ \hline
    Right occipital & O2, P8\\ \hline
  \end{tabular}
\end{table}
